# Supplementary material for: Deep Layer Aggregation
Source: arXiv:1707.06484 source file (2019-01-04)
Supplement: Supplementary file 1 [file appendix.tex]

\section{ImageNet Classification}

The concept of DLA framework is general since it doesn't require particular designs of convolution blocks. We also turn to simple design of aggregation nodes in our applications. Figure~\ref{fig:nodes} shows the aggregation nodes for hierarchical aggregation. It is a concatenation of the input channels followed by a 1 $\times$ 1 convolution. We explore adding residual connection in the aggregation as shown in Figure~\ref{fig:nodes}(c). It is only used when there are more than 100 layers in the classification network. Three types of convolutional blocks are studied in this paper, as shown in Figure~\ref{fig:blocks}, since they are widely used in deep learning literature. Because the convolutional blocks will be combined with additional linear projection in the aggregation nodes, we reduce the ratio of bottleneck blocks from 4 to 2. 

\begin{comment}
\begin{figure}[htp]
    \centering
    \includegraphics[width=\linewidth]{fig/fig-imagenet-multiadd.pdf}
    % \includegraphics[width=\linewidth]{tab/fig-imagenet.pdf}
    % \begin{subfigure}{0.4\textwidth}
    % % \includegraphics[width=\linewidth]{fig/imagenet_params}
    % \includegraphics[width=\linewidth]{tab/fig-imagenet-params.pdf}
    % \end{subfigure}
    %     \begin{subfigure}{0.4\textwidth}
    % \includegraphics[width=\linewidth]{tab/fig-imagenet-multiadd.pdf}
    % %  \includegraphics[width=\linewidth]{fig/imagenet_gflops}
    %      \end{subfigure}

    \caption{
    Evaluation of DLA on ILSVRC.
    DLA/DLA-X have ResNet/ResNeXT backbones respectively.
    DLA achieves the highest accuracies with fewer computation.
    }
    \label{fig:imagenet_flops}
\end{figure}

\end{comment}

\begin{figure*}[hbt]
	\centering
	\ra{1.2}
	\adjustbox{max width=\columnwidth}{
		\begin{tabular}{c c c}
			\includegraphics[height=0.65in]{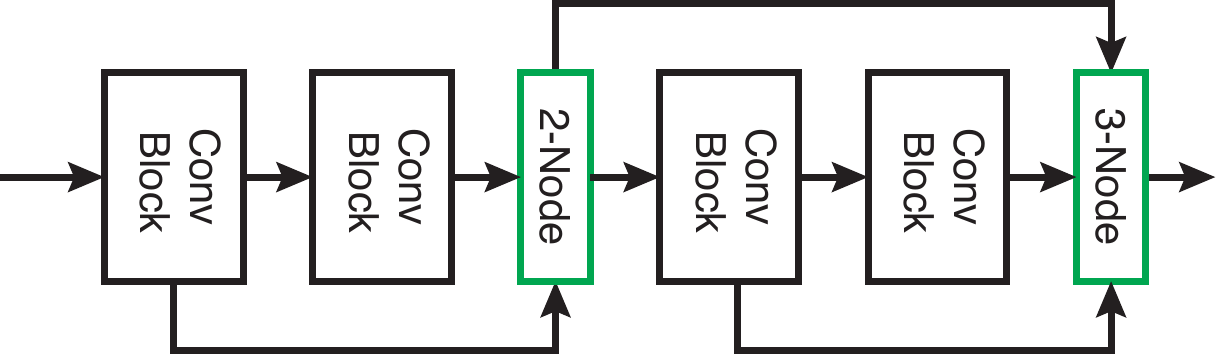} & \includegraphics[height=0.65in]{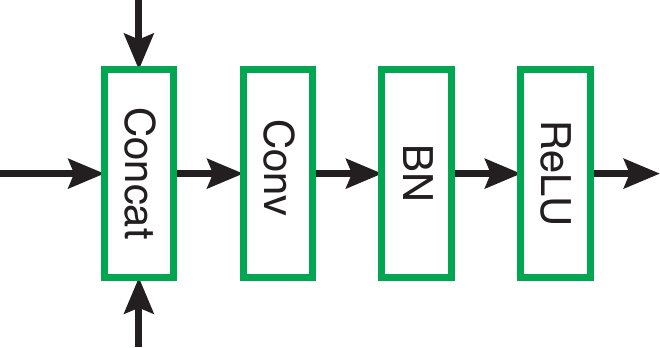} & \includegraphics[height=0.65in]{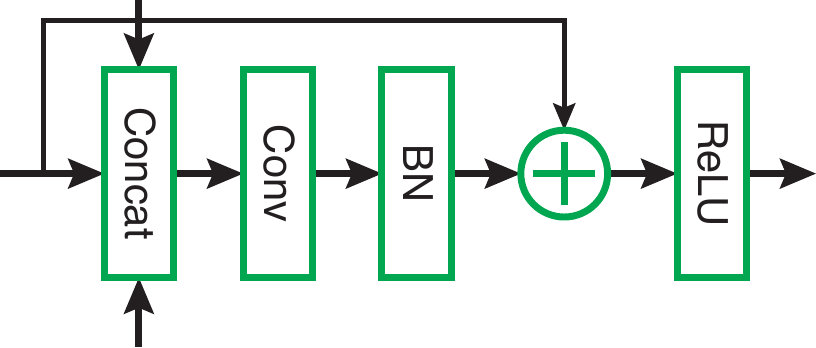} \\
			{\small (a) 3-level hierarchical aggregation} & {\small (b) Plain 3-node} & {\small (c) Residual 3-node}
		\end{tabular}}
		\caption{Illustration of
		aggregation node architectures.
		%(a) shows another view of HDA.
		%(b) and (c) show two general designs of nodes with 3 inputs.
		%In (b), the inputs are concatenated and passed to a convolutional layer.
		%In (c), after batch normalization, an additional residual connection adds input from the last block to the node output to improve gradient propagation.
		}
		\label{fig:nodes}
\end{figure*}

\begin{figure*}[htb]
	\centering
	\ra{1.2}
	\adjustbox{max width=\columnwidth}{
		\begin{tabular}{c c c}
			\includegraphics[height=0.6in]{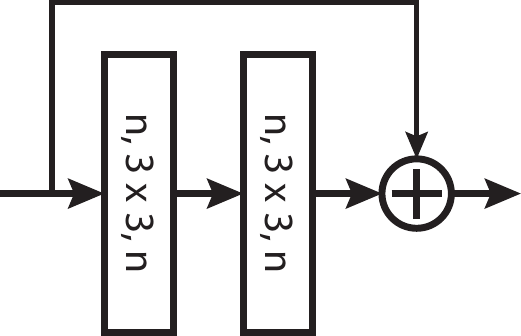} & \includegraphics[height=0.6in]{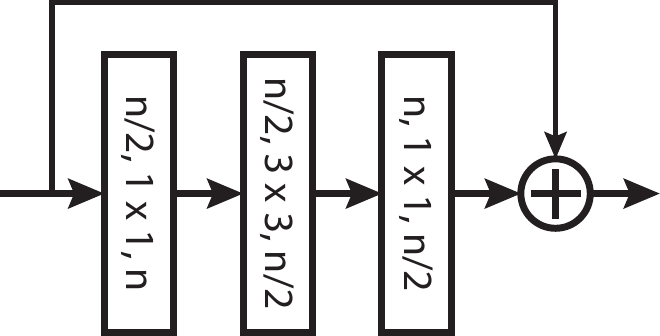} & \includegraphics[height=0.6in]{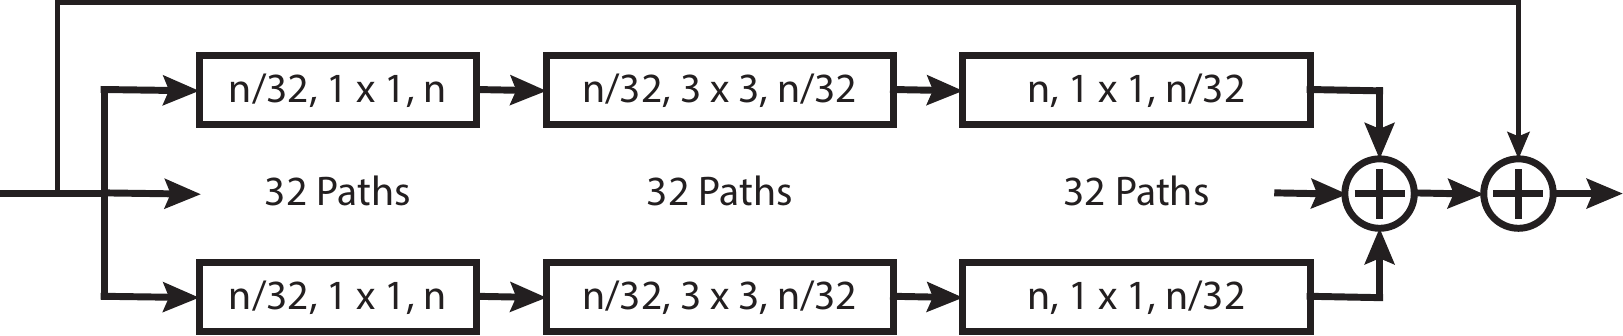} \\
			{\small (a) Basic} & {\small (b) Bottleneck} & {\small (c) Split}
		\end{tabular}}
		\caption{Convolutional blocks used in this paper. Our aggregation architecture is as general as stacking layers, so we can use the building blocks of existing networks. The layer labels indicate output channels, kernel size and input channels. (a) and (b) are derived from~\cite{he2016deep} and (c) from~\cite{xie2016aggregated}.}
		\label{fig:blocks}.
\end{figure*}

We compare DLA and DLA-X to other networks in Figure 5 in the submitted paper in terms of network parameters and classification accuracy. DLA includes the networks using residual blocks in ResNet and DLA-X includes those using the block in ResNeXt. For fair comparison, we design DLA and DLA-X networks with similar depth and channels with their counterparts. The ResNet models are ResNet-34, ResNet-50, ResNet-101 and ResNet-152. The corresponding DLA model depths are 34, 60, 102, 169. The ResNeXt models are ResNeXt-50 (32x4d), ResNeXt-101 (32x4d), and ResNeXt-101 (64x4d). The corresponding DLA-X model depths are 60 and 102, while the third DLA-X model double the number of 3 $\times$ 3 bottleneck channels, similar to ResNeXt-101 (64x4d). 
% In addition to comparison of parameters and accuracy, Figure~\ref{fig:imagenet_flops} also compares the relation between computation and accuracy. It shows that DLA models also achieve advantageous computation efficiency.

\section{Semantic Segmentation}

% \begin{figure*}[htp]
%     \centering
%      \includegraphics[width=\linewidth]{tab/fig-imagenet.pdf}
%     \caption{Comparison of DLA with other models in terms of parameter efficiency on ILSVRC}
%     \label{fig:imagenet}
% \end{figure*}

% \input{tab/table_finegrained}

\begin{table*}[htbp]
\centering
\ra{1.2}
\adjustbox{max width=\linewidth}{
\small
\begin{tabular}{l c c c c c c c c c c c c c} %{l||c|c|c|c|c|c|c|c|c|c|c||c}
%\begin{tabular}{@{}l@{\hspace{5mm}}*{11}{@{\hspace{2mm}}c}@{\hspace{5mm}}c@{\hspace{2mm}} c}
    & \ver{Data Aug} & \ver{Building} & \ver{Tree} & \ver{Sky} & \ver{Car} & \ver{Sign} & \ver{Road} & \ver{Pedestrian} &
    \ver{Fence} & \ver{Pole} & \ver{Sidewalk} & \ver{Bicyclist} & \ver{mean IoU} \\ \hline
% ALE
% \cite{russell2009associative} & & 73.4 & 70.2 & {91.1} & 64.2 & 24.4 & 91.1 & 29.1 & 31.0 &
% 13.6 & 72.4 & 28.6 & 53.6 \\
% SuperParsing
% \cite{tighe2010superparsing} & &70.4 & 54.8 & 83.5 & 43.3 & 25.4 & 83.4 & 11.6 & 18.3
% & 5.2 & 57.4 & 8.9 & 42.0 \\
% Liu and He
% \cite{liu2015multiclass} & & 66.8 & 66.6 & 90.1 & 62.9 & 21.4 & 85.8 & 28.0 & 17.8 &
% 8.3 & 63.5 & 8.5 & 47.2 \\
% SegNet
% \cite{badrinarayanan2015segnet} & & 68.7 & 52.0 & 87.0 & 58.5 & 13.4 & 86.2 & 25.3 & 17.9 & 16.0
% & 60.5 & 24.8 & 46.4 \\
% DeepLab-LFOV
% \cite{chen2014semantic} & & 81.5 & 74.6 & 89.0 & 82.2 & 42.3 & {92.2} & 48.4 & 27.2 & 14.3 & {75.4} & 50.1 & 61.6 \\
% Dilation8
% \cite{yu2016multi} & & {82.6} & {76.2} & 89.9 & {84.0} & {46.9} & {92.2} & {56.3} & {35.8} & {23.4} & 75.3 & {55.5} & {65.3} \\
% FSO \cite{kundu2016feature} & & 84.0 & 77.2 & 91.3 & 85.6 & 49.9 & 92.5 & 59.1 & 37.6 & 16.9 & 76 & 57.2 & 66.1 \\ \hline

DLA-34 8s & \multirow{5}{*}{No} & 83.2 & 77.2 & 91.2 & 83.6 & 48.8 & 94.3 & 58.6 & 32.0 & 27.8 & 81.1 & 55.4 & 66.7 \\
DLA-60 8s & & 83.0 & 77.0 & 91.4 & 84.1 & 46.9 & 94.1 & 58.3 & 32.8 & 26.0 & 81.3 & 56.8 & 66.5 \\
DLA-34 & & 83.2 & 76.4 & 92.5 & 84.6 & 52.1 & 94.4 & 61.5 & 29.4 & 35.1 & 82.0 & 57.8 & 68.1 \\
DLA-60 & & 84.4 & 77.7 & 92.6 & 87.1 & 51.4 & 95.3 & 62.2 & 32.1 & 36.2 & 84.5 & 64.1 & 69.8 \\
DLA-102 & & 84.9 & 78.0 & 92.5 & 86.4 & 50.8 & 94.9 & 62.8 & 45.4 & 35.7 & 83.7 & 65.8 & 71.0 \\ \hline
DLA-60 &  \multirow{3}{*}{Yes} & 86.6 & 79.3 & 92.5 & 90.9 & 55.3 & 96.2 & 65.5 & 48.6 & 37.4 & 86.9 & 66.5 & 73.2 \\
DLA-102 & & 86.6 & 78.8 & 92.2 & 90.3 & 57.9 & 96.5 & 66.7 & 49.6 & 38.7 & 87.9 & 66.7 & 73.8 \\
DLA-169 & & 86.9 & 78.9 & 92.5 & 89.9 & 58.5 & 96.5 & 66.1 & 55.4 & 39.0 & 87.7 & 67.7 & 74.4 \\ \hline

\end{tabular}
}
\caption{Semantic segmentation results on the CamVid dataset.}
%  \vspace{-3mm}
% \vspace{-2mm}
\label{tab:camvid}
\end{table*}

\begin{table*}[h!btp]
\centering
\ra{1.2}
\adjustbox{max width=\linewidth}{
\small
 \begin{tabular}{@{}l@{\hspace{5mm}}*{19}{@{\hspace{2mm}}c}@{\hspace{5mm}}c@{\hspace{2mm}} c}
 &  \ver{Road} & \ver{Sidewalk} & \ver{Building} & \ver{Wall} &
    \ver{Fence} & \ver{Pole} & \ver{Light} & \ver{Sign} & \ver{Vegetation} & \ver{Terrain} & \ver{Sky} & \ver{Person} & \ver{Rider}
    & \ver{Car} & \ver{Truck} & \ver{Bus} & \ver{Train} &
    \ver{Motorcycle} & \ver{Bicycle} & \ver{mean IoU} \\
 \midrule
    DLA-34 8s & 97.9 & 83.2 & 91.9 & 47.7 & 57.7 & 62.4 & 68.6 & 77.3 & 92.2 & 60.4 & 94.8 & 81.1 & 59.8 & 94.1 & 57.5 & 76.6 & 54.2 & 59.7 & 76.6 & 73.4 \\
% DLA-60 8s & 97.8 & 82.9 & 91.8 & 45.7 & 55.7 & 63.3 & 70.3 & 79.3 & 92.3 & 60.9 & 95.0 & 81.8 & 60.0 & 94.1 & 50.0 & 75.8 & 51.6 & 60.6 & 77.5 & 73.0 \\ \midrule
DLA-34 & 98.0 & 83.5 & 92.1 & 51.0 & 56.8 & 64.9 & 69.6 & 78.5 & 92.4 & 62.9 & 95.1 & 81.5 & 59.6 & 94.5 & 59.0 & 78.4 & 57.8 & 62.9 & 76.9 & 74.5 \\
% DLA-60 & 97.9 & 83.4 & 91.7 & 40.4 & 55.7 & 65.5 & 70.8 & 79.9 & 92.4 & 60.7 & 95.1 & 82.1 & 60.2 & 94.3 & 50.1 & 77.4 & 47.2 & 61.2 & 77.9 & 72.8 \\
DLA-102 & 98.0 & 84.3 & 92.3 & 43.2 & 56.9 & 67.2 & 71.6 & 80.9 & 92.5 & 61.4 & 94.6 & 82.7 & 61.5 & 94.5 & 60.3 & 77.7 & 53.8 & 62.2 & 78.5 & 74.4 \\
DLA-169 & 98.2 & 84.8 & 92.5 & 45.9 & 60.0 & 68.0 & 72.3 & 81.1 & 92.7 & 61.9 & 95.1 & 83.4 & 63.3 & 95.3 & 70.9 & 80.8 & 48.1 & 65.4 & 79.1 & 75.7 \\
\midrule
DLA-34 MS & 98.2 & 84.7 & 92.5 & 54.3 & 59.5 & 65.9 & 71.1 & 79.5 & 92.7 & 64.1 & 95.3 & 82.6 & 61.8 & 94.7 & 63.3 & 83.7 & 64.6 & 64.2 & 77.6 & 76.3 \\

% DLA-60 MS & 98.1 & 84.6 & 92.1 & 43.5 & 58.2 & 66.4 & 71.8 & 81.0 & 92.7 & 62.6 & 95.3 & 83.0 & 61.2 & 94.5 & 53.5 & 82.0 & 53.0 & 64.8 & 78.9 & 74.6 \\

DLA-102 MS & 98.5 & 85.0 & 92.5 & 47.1 & 56.7 & 66.9 & 74.4 & 78.6 & 93.6 & 71.7 & 95.1 & 85.8 & 67.4 & 95.3 & 55.8 & 63.5 & 57.8 & 68.1 & 76.1 & 76.1 \\
DLA-169 MS & 98.3 & 85.9 & 92.8 & 48.3 & 61.2 & 69.0 & 73.4 & 82.2 & 92.9 & 63.1 & 95.4 & 84.2 & 65.1 & 95.7 & 76.3 & 82.9 & 49.6 & 68.5 & 80.2 & 77.1 \\

\midrule

 \end{tabular}
}
\vspace{-1mm}
 \caption{
 Performance of DLA on the Cityscapes validation set. s8 indicates the input image is downsampled by 8 in the model output. It is 2 by default. Lower downsampling rate usually leads to higher accuracy. 
 ``MS'' indicates the models are tested on on multiple scales of the input images.
 %We also find that DLA-34 has very good performance despite its smaller number of layers. We also test the models on multiple scales of the input images, same as the testing procedure of the previous works. Those methods are marked by ``MS''.
 % MS means multi-scale testing.
 % Method marked with $\dagger$ used IDA to upsample the prediction results, while the other methods use bilinear interpolation to upsample the feature maps that are 8$\times$ smaller than input images in spatial resolution.
 % The additional parameters for IDA upsampling is negligible.
 % DRN-26 and DRN-42 are in DRN-C family proposed by \cite{yu2017dilated}}
 % TODO scope these results: no context models, no ensembles, etc. [ES]
 }
\label{tab:cityscapes}
\end{table*}

We report experiments for semantic segmentation on CamVid and Cityscapes. Table~\ref{tab:camvid} shows a breakdown of the accuracies for the categories. We also add data agumention in the CamVid training, as shown in the third group of Table~\ref{tab:camvid}. It includes random rotating the images between -10 and 10 degrees and random scaling between 0.5 and 2. We find the results can be further improved by the augmentation. Table~\ref{tab:cityscapes} shows the breakdown of categories in Cityscapes on the validation set. We also test the models on multiple scales of the images. This testing procedure is used in evaluating the models on the testing images in the previous works.
